# Supplementary material for: Spectral Gradient Iterative Edge Attack for Synchronization Suppression in Complex Networks
Source: arXiv:2505.06489 source file (2026-10-03)
Supplement: Supplementary file 1 [file Supplementary1.tex]

\appendix

 % Laplacian matrix

\subsection{Numerical Verification}
In order to verify the accuracy of our conclusion, that is, for some classical network models, the first-order attack strategy is completely consistent with the real situation, Pearson correlation coefficient in this issue is defined as 
\begin{align}
    \text{Person correlation  }(\rho) = \frac{\text{Edges with first-order ranking}}{\text{Real edge ranking}}.
\end{align}
The results (tab.\ref{tab:accuracy}) shows the unmatched accuracy FIA in Scale-Free (BA), Random (ER) and Small-World (WS) network.
\begin{table}[h]
    \centering
    \caption{(Spearman  $\rho$ ) in different typical networks}
    \label{tab:accuracy}
    \begin{tabular}{lc}
        \toprule
        \textbf{Network Generation}& \textbf{Spearman correlation $\rho$}\\
        \midrule
        BA Network (n=100, m=60)&0.9998\\
        BA Network (n=1000, m=6)& 0.9970\\
        BA Network (n=5000, m=10)& 0.9979\\
        \midrule
        ER Network (n=100, p=0.06)&0.9987\\
        ER Network (n=1000, p=0.006)& 0.9991\\
        ER Network (n=5000, p=0.01)& 1.0000\\
        \midrule
        WS Network (n=100, k=10, p=0.8)&0.9972\\
        WS Network (n=1000, k=6, p=0.1)& 0.9998\\
        WS Network (n=5000, k=10, p=0.1)& 0.9999\\
        \bottomrule
    \end{tabular}
\end{table}

\section{Compared Removal Algorithm}
\label{sec:degree-algo}

The algorithm iteratively removes edges while preserving network connectivity through three phases:

\begin{enumerate}
    \item \textbf{Initialization}: Create graph copy $G_{\text{temp}} \gets G$
    
    \item \textbf{Iterative Removal}:
    \begin{itemize}
        \item Compute node degrees $\{d_i\}$ for $G_{\text{temp}}$
        \item Rank edges by descending degree difference $|d_i - d_j|$
        \item Attempt removal of top-ranked edge:
        \begin{equation}
            Tar^*(i,j) = \arg\max_{(u,v)\in E} |d_i - d_j|
        \end{equation}
        \item If removal preserves connectivity: accept $e^*$, else test lower-ranked edges
    \end{itemize}
    
    \item \textbf{Termination}: Stop when no removable edges exist
\end{enumerate}

\textbf{Complexity Analysis}:
\begin{itemize}
    \item Time per iteration: $\mathcal{O}(m\log m)$ (sorting dominates)
    \item Connectivity check: $\mathcal{O}(m+n)$ per edge trial
    \item Worst-case total: $\mathcal{O}(Tm\log m)$ for $T$ removed edges
\end{itemize}

\textbf{Key Advantages}:
\begin{itemize}
    \item Avoids costly spectral computations
    \item Requires only local degree information
    \item Guarantees connectivity via validation step
\end{itemize}

 \begin{table}[htbp]
\centering
\caption{the definition of compared algorithm}
\label{tab:complexity}
\begin{tabular}{ll}
\hline
\textbf{Metric (Abbr.)} & \textbf{Algorithm Description} \\ \hline
Degree (Deg) & Select edges with maximum node degree difference \\
Betweenness (Bet) & Edge selection by Brandes' betweenness centrality \\ 
Closeness (Clos) & Select edges connecting nodes with maximum closeness difference \\
Eigenvector (Eig) & Power iteration for eigenvector centrality difference \\
PageRank (PR) & Iterative PageRank difference calculation \\ \hline
\end{tabular}
\end{table}
