# Supplementary material for: Spectral Gradient Iterative Edge Attack for Synchronization Suppression in Complex Networks
Source: arXiv:2505.06489 source file (2026-10-03)
Supplement: Supplementary file 2 [file Supplementary2.tex]

\section{Second-Order Perturbation Derivation for Fiedler Value} \label{app:perturb}

\subsection{Problem Setup}
Consider a network depicted by $\lap \in \mathbb{R}^{n\times n}$ as symmetric Laplacian matrix, $\lambda_2$ as  Fiedler value (smallest nonzero eigenvalue),  $\vect{x} \in \mathbb{R}^n$ as Fiedler vector  and using $\Delta\lap$ to represent perturbation matrix due to edge removal.

\subsection{First-Order Perturbation} \label{app:first}
The perturbed eigenvalue equation:
\begin{equation}
    (\lap + \Delta\lap)(\vect{x} + \delta\vect{x}) = (\lambda_2 + \delta\lambda_2)(\vect{x} + \delta\vect{x}).
\end{equation}
Expanding to first order and left-multiplying by $\vect{x}^\top$and considering $\vect{x}$ is unit eigenvector, that is,  $\|\vect{x}\|=1$, we have
\begin{align}
    \vect{x}^\top\lap\delta\vect{x} + \vect{x}^\top\Delta\lap\vect{x} &= \lambda_2\vect{x}^\top\delta\vect{x} + \delta\lambda_2 \vect{x}^\top\vect{x}.
\end{align}
Using $\lap\vect{x} = \lambda_2\vect{x}$ and $\vect{x}^\top\vect{x} = 1$,
\begin{equation}
    \delta\lambda_2^{(1)} = \vect{x}^\top\Delta\lap\vect{x} ,\label{eq:first_order}
\end{equation}
which demonstrates that the first-order correction depends linearly on the perturbation through the Fiedler vector.

Now we come to consider edge removal specific form. Based on the features of Laplacian matrix, for removal of edge $e_{ij}$:
\begin{equation}
    \Delta\lap = -(\vect{e}_i - \vect{e}_j)(\vect{e}_i - \vect{e}_j)^\top \label{eq:deltaL}
\end{equation}
where $\vect{e}_k$ is the standard basis vector. Substituting \eqref{eq:deltaL} into \eqref{eq:first_order}:
\begin{align}
    \delta\lambda_2^{(1)} &= -(x_i - x_j)^2 \label{eq:first_result}
\end{align}
which shows the edges bridging nodes with largest Fiedler vector differences ($|x_i - x_j|$) make most contribution to $\lambda_2$.

\subsection{Second-Order Correction} \label{app:second}
To further clarify the effect of edge on synchronization performance in the network, the eigenvector perturbation $\delta\vect{x}$ can be expanded as:
\begin{equation}
    \delta\vect{x} = \sum_{k\neq2} c_k \vect{x}_k \label{eq:eigen_expansion}
\end{equation}
where $\vect{x}_k$ are other eigenvectors satisfying $\lap\vect{x}_k = \lambda_k\vect{x}_k$.

Substituting \eqref{eq:eigen_expansion} into \eqref{eq:first_order} and projecting onto $\vect{x}_m$ ($m\neq2$):
\begin{align}
    c_m &= \frac{\vect{x}_m^\top\Delta\lap\vect{x}}{\lambda_2 - \lambda_m} \label{eq:cm}
\end{align}

The second-order correction comes from:
\begin{align}
    \delta\lambda_2^{(2)} &= \sum_{k\neq2} \frac{(\vect{x}^\top\Delta\lap\vect{x}_k)^2}{\lambda_2 - \lambda_k} \label{eq:second_general}
\end{align}

\subsection{Dominant Term Selection} \label{app:dominant}
Under the spectral gap condition $\lambda_3 - \lambda_2 \ll \lambda_k - \lambda_2$ ($k\geq4$), the dominant contribution comes from $\lambda_3$:
\begin{align}
    \delta\lambda_2^{(2)} &\approx \frac{(\vect{x}^\top\Delta\lap\vect{x}_3)^2}{\lambda_2 - \lambda_3} \label{eq:second_approx}
\end{align}

Substituting $\Delta\lap$ from \eqref{eq:deltaL}:
\begin{align}
    \vect{x}^\top\Delta\lap\vect{x}_3 &= -(x_i - x_j)(x_{3,i} - x_{3,j}) \label{eq:inner_product}
\end{align}

Final second-order term:
\begin{equation}
    \delta\lambda_2^{(2)} \approx \frac{(x_i - x_j)^2(x_{3,i} - x_{3,j})^2}{\lambda_3 - \lambda_2} \label{eq:second_final}
\end{equation}

\textbf{Interpretation:} The second-order correction amplifies the attack effect through coupling with the third eigenmode.

\subsection{Total Perturbation} \label{app:total}
Combining \eqref{eq:first_result} and \eqref{eq:second_final}:
\begin{equation}
    \delta\lambda_2 \approx -(x_i - x_j)^2 - \frac{(x_i - x_j)^2(x_{3,i} - x_{3,j})^2}{\lambda_3 - \lambda_2} \label{eq:total_perturb}
\end{equation}

\begin{itemize}
    \item \textbf{Leading term}: Linear suppression proportional to $(x_i - x_j)^2$
    \item \textbf{Higher-order term}: Nonlinear enhancement when $(x_i - x_j)^2(x_{3,i} - x_{3,j})^2$ dominates
\end{itemize}

\subsection{Physical Interpretation}
\begin{itemize}
    \item \textbf{Spectral gap $\gamma$}: Larger $\gamma$ suppresses second-order effects
    \item \textbf{Mode correlation $\beta$}: Weak coupling ($\beta \ll 1$) maintains hierarchy
    \item \textbf{Typical networks}: Scale-free and small-world networks satisfy $\beta \sim O(10^{-2})$, $\gamma \sim O(1)$
\end{itemize}
